# Supplementary material for: Multistability and High Codimension Bifurcations in Synergistic Epidemics on Heterogeneous Networks
Source: arXiv:2504.13293 ancillary file (2025-07-07)
Supplement: Supplementary file 1 [file SM.pdf]

# Supplemental Material for "Multistability and High Codimension Bifurcations in Synergistic Epidemics on Heterogeneous Networks"

Francisco J. Pérez-Reche
*School for Natural and Computing Sciences, University of Aberdeen, Aberdeen, UK*[*]

Sergei N. Taraskin
*St. Catharine's College and Department of Chemistry, University of Cambridge, Cambridge, UK*[†]

## I. POSSIBLE REGIMES FOR NON-SYNERGISTIC EPIDEMICS

Within the single-site heterogeneous mean-field (SSHMF) approximation, it can be rigorously proven that non-synergistic epidemics ($\beta = 0$) can only exhibit regimes I and II, irrespective of the node degree distribution. This follows from the fact that only a transcritical bifurcation of type TC$^-$ is possible for $\beta = 0$.

This can be established from the following theorem:

**Theorem I.1.** *TC$^+$ and SN$^\pm$ bifurcations cannot occur for synergy-free SIS processes with $\beta = 0$.*

*Proof.* The proof relies on the fact that the second derivative, $F^{(2)}(\theta)$, of the function $F(\theta)$ (Eq. (6) in the main text), which is given by the following expression for $\beta = 0$,

$$F^{(2)}(\theta) = \begin{cases} -\frac{\mu\alpha^2}{\langle k\rangle}\left\langle \frac{k^2(k-1)(1-\theta\alpha)^{k-2}}{[\mu+1-(1-\theta\alpha)^k]^2} + \frac{2k^3(1-\theta\alpha)^{2k-2}}{[\mu+1-(1-\theta\alpha)^k]^3}\right\rangle & \text{with } q_k(\theta) = 1-(1-\alpha\theta)^k \quad \text{for d-time}, \\ -\frac{2}{\langle k\rangle}\left(\frac{\alpha}{\mu}\right)^2\left\langle \frac{k^3}{[1+(\alpha/\mu)k\theta]^3}\right\rangle & \text{with } q_k(\theta) = \alpha k\theta \quad \text{for c-time}, \end{cases} \tag{1}$$

is negative $\forall\theta \in [0,1]$ given $\alpha \in (0,1]$ and $\mu \in (0,1]$ for d-time, and $\alpha,\mu \in (0,\infty)$ for c-time. In other words, $F(\theta)$ is concave for synergy-free epidemics. In Eq. (1), the identity $\lambda_n \equiv \alpha$ holding for $\beta = 0$ has been used. For briefness, the dependence of $F$ on the model parameter set $\Gamma$ is omitted in this section.

Since $F^{(2)}(0) < 0$, the transcritical bifurcation TC$^+ = \mathcal{B}_1^+(0)$ cannot occur, since such a bifurcation requires $F^{(2)}(0) > 0$ (see Eq. (7) of the main text).

A similar argument rules out the possibility of an SN$^+ = \mathcal{B}_1^+(\theta_*)$ bifurcation at some $\theta_* \in (0,1)$.

The impossibility of an SN$^- = \mathcal{B}_1^-(\theta_*)$ bifurcation at $\theta_* \in (0,1)$ can be proven by contradiction.

Assume that SN$^-$ exists, which means that $F(\theta_*) = F^{(1)}(\theta_*) = 0$ and $F^{(2)}(\theta_*) < 0$ (see Eq. (7) of the main text).

Since $F(\theta_*) = F^{(1)}(\theta_*) = 0$, Rolle's theorem guarantees the existence of at least one point $c \in (0,\theta_*)$ where $F^{(1)}(c) = 0$ [1].

At the same time, since $F^{(2)}(\theta) < 0$ for all $\theta \in [0,1]$, the function $F^{(1)}(\theta)$ is strictly decreasing in $\theta \in [0,1]$. This implies that for any $\theta > c$, we must have $F^{(1)}(\theta) < 0$. In particular, for $\theta_* > c$, we obtain $F^{(1)}(\theta_*) < 0$, which contradicts the assumption that $F^{(1)}(\theta_*) = 0$ necessary for an SN$^-$ bifurcation.

Thus, such a bifurcation cannot occur meaning none of the TC$^+$ and SN$^\pm$ bifurcations can occur as stated by the theorem. □

**Corollary I.1.1.** *No codimension-$\bar{d}$ bifurcations can occur for synergy-free SIS processes with $\bar{d} > 1$.*

Referring to the graph representation of dynamical regimes shown in Fig. 1 of the main text, the impossibility of the bifurcations TC$^+$ and SN$^\pm$ implies that no transition to other regimes III-IV is possible from regimes I and II, as this would require crossing the bifurcations TC$^+$ or SN$^\pm$ when varying the values of the parameters of the model.

[*] fperez-reche@abdn.ac.uk
[†] snt1000@cam.ac.uk

This restriction extends beyond codimension-1 bifurcations. Since bifurcations $SN^{\pm}$ do not exist for $\beta = 0$, no higher-codimension bifurcations can occur, as they ultimately arise from interactions involving SN bifurcations.

## II. CODIMENSION-3 AND 4 BIFURCATIONS

In this subsection, we show the invasion curves $p(\alpha)$ in binary graphs that exhibit bifurcations of codimension-3 and 4. The results are are obtained within the SSHMF approximation. There are two types of codimension-3 bifurcations: CSNT (cusp-(saddle-node-transcritical) crossing point) and CC (cusp-cusp crossing point) bifurcations. The CSNT and CC bifurcations correspond to the appearance of four degenerate roots of $F(\theta)$ at $\theta = \theta_* = 0$ and $\theta = \theta_* \in (0, 1)$, respectively. The loci of the CSNT and CC bifurcations are represented by solid and dashed curves, respectively, in the $(\mu, \varphi)$ parameter space for BG, as shown in Fig. 2(a) of the main text and in the insets of panels (b) and (e) of Fig. 1. As seen from these figures, the CC curve merges with the CSNT curve at a single point marked by star which represents the codimension-4 bifurcation point, $CCCSNT^{-}$, i.e. (cusp-cusp)-(cusp-saddle-node-transcritical) crossing point. This codimension-4 bifurcation corresponds to the appearance of five-degenerate trivial roots of $F(\theta)$ (see Fig. 1(a)).

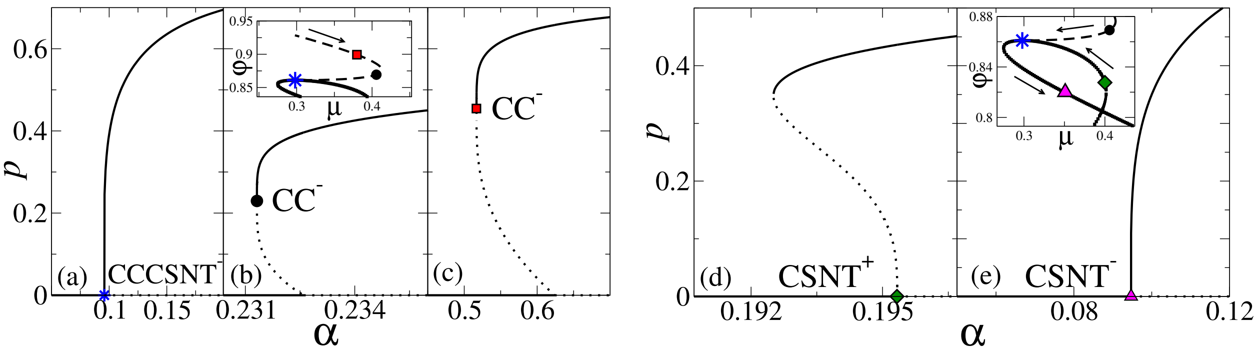


FIG. 1: Invasion curves $p(\alpha)$ in BG(10,30,$\varphi$) at: (a) $(\beta, \varphi, \mu) \simeq (-0.104, 0.861, 0.298)$ with $\alpha_* = \alpha_4 \simeq 0.096$ and $p_* = p(\alpha_*) = 0$ at the $CCCSNT^{-}$ bifurcation (star); (b) $(\beta, \varphi, \mu) \simeq (-0.159, 0.869, 0.406)$ with $\alpha_* \simeq 0.231$ and $p_* \simeq 0.23$ at $CC^{-}$ bifurcation (circle); (c) $(\beta, \varphi, \mu) \simeq (-0.279, 0.899, 0.38)$ with $\alpha_* \simeq 0.517$ and $p_* \simeq 0.455$ at the $CC^{-}$ bifurcation (square); (d) $(\beta, \varphi, \mu) \simeq (-0.135, 0.828, 0.4)$ with $\alpha_* \simeq 0.195$ and $p_* = 0$ at the $CSNT^{+}$ bifurcation (diamond); (e) $(\beta, \varphi, \mu) \simeq (-0.087, 0.82, 0.351)$ with $\alpha_* \simeq 0.095$ and $p_* = 0$ at the $CSNT^{-}$ bifurcation (triangle). The insets in (b) and (e) show the locations of the codimension-3 and codimension-4 bifurcation points in the $(\mu, \varphi)$ parameter space, as displayed in Fig. 2(a) of the main text.

All points in the CC bifurcation curve are of type $CC^{-}$ because the maximum number of roots of $F(\theta)$ does not exceed five and one of the roots is located at $\theta_* = 0$ (see Fig. 1(b)-(c)). Bifurcations of type $CC^{+}$ would require a higher number of roots. The value of the finite four-degenerate root $\theta_*$ (and thus the value of $p_* = p(\theta_*)$) for $CC^{-}$ bifurcation on the dashed lines approaches zero when it moves along the curve in the direction indicated by the arrow in the insets of panels (b) and (e) of Fig. 1 and reaches zero at the $CCCSNT^{-}$ bifurcation point (see sequentially panels (c), (b) and (a) in Fig. 1). In contrast, the type of CSNT bifurcation depends on the position of the bifurcation point on the CSNT bifurcation curve. If we follow the solid line along the arrows shown in the inset of panel (e) in Fig. 1 then $F^{(4)}(0) > 0$ and the bifurcations are of $CSNT^{+}$ type before the $CCCSNT^{-}$ bifurcation point is reached (see Fig. 1(d)). After passing the $CCCSNT^{-}$ bifurcation, the CSNT bifurcation changes its type and becomes $CSNT^{-}$ (see Fig. 1(e)). In fact, the $CSNT^{+}$ and $CC^{-}$ bifurcations collide at the $CCCSNT^{-}$ bifurcation and then transform to the $CSNT^{-}$ bifurcation (when following the direction of the arrows shown in the inset of panel(e)).

## III. SYNERGISTIC EPIDEMICS IN REAL NETWORKS

In this subsection, we present the results of the SSHMF analysis of synergistic SIS epidemics spreading in two real networks: the Douban social network [2] and the Western US power grid [3]. Both real networks exhibit similar bifurcation diagrams. We start with analysis of the Douban network.

Fig. 2 shows the bifurcation diagrams for continuous-time (c-time, panel (a)), and discrete-time (d-time, panel (b)). For a given network topology with a fixed subset $\Gamma_N$ of network parameters, which is the case for any real network, the

set of relevant parameters $\Gamma$ is reduced from $\{\alpha, \beta, \mu, \Gamma_N\}$ to $\{\tilde{\alpha}, \beta\}$ with $\tilde{\alpha} = \alpha/\mu$ in the case of c-time dynamics and to $\{\alpha, \beta, \mu\}$ in the case of d-time dynamics. The number of parameters determines the number of different bifurcation points which might appear in the parameter space. For example, for c-time dynamics, there are only two parameters and thus typically bifurcations of codimension-1 and codimension-2 could be found in the bifurcation diagrams in the $(\tilde{\alpha}, \beta)$ parameter space. Such a situation is illustrated in Fig. 3, where all types of bifurcations of codimension-1 and SNT bifurcations of codimension-2 are present. This bifurcation diagram resembles panel (b) of Fig. 2 in the main text, although the number of SNT bifurcations and the number of dynamical regimes is reduced to two and four, respectively, for the Douban network, compared to the bifurcation diagram for the binary graph shown in the main text.

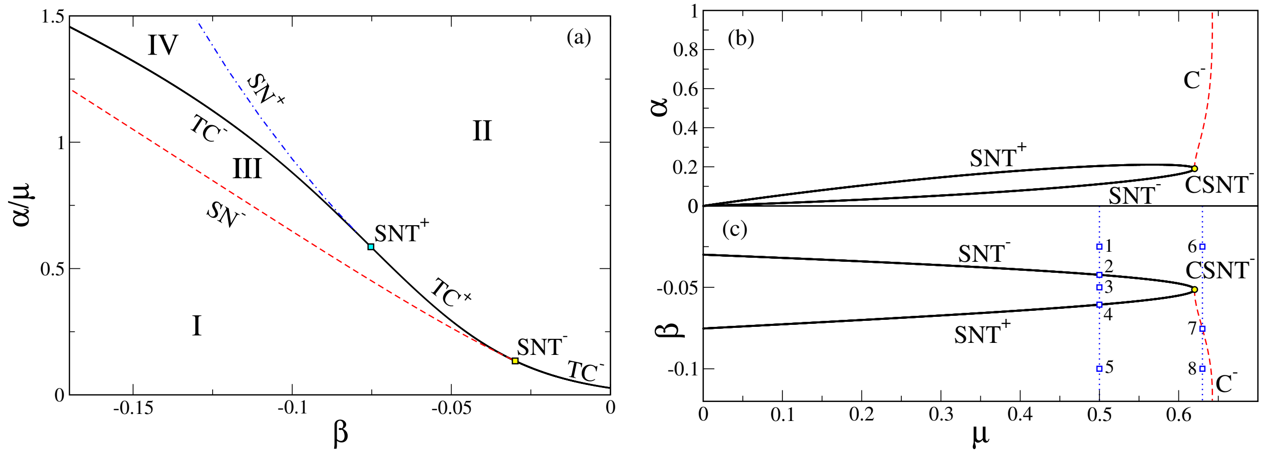


FIG. 2: Bifurcation diagrams for synergistic SIS epidemics spreading on the Douban network. Panel (a) shows in $(\alpha/\mu, \beta)$ parameter space the loci for the $TC^{\pm}$ (solid curve), $SN^{-}$ (dashed), $SN^{+}$ (dot-dashed) and $SNT^{\pm}$ (squares) bifurcations for c-time dynamics within the SSHMF approximation. Different dynamical regimes are indicated by I-IV.
Panels (b) and (c) show in $(\alpha, \mu)$ and $(\beta, \mu)$ parameter spaces, respectively, the loci for the $SNT^{\pm}$ (solid curve), $C^{-}$ (dashed) and $CSNT^{-}$ (circles) bifurcations for SIS in the d-time regime obtained within the SSHMF approximation. The numbered squares on two dotted lines indicate the specific values of parameter pairs $(\beta, \mu)$ corresponding to the invasion curves with matching labels in Fig. 3.

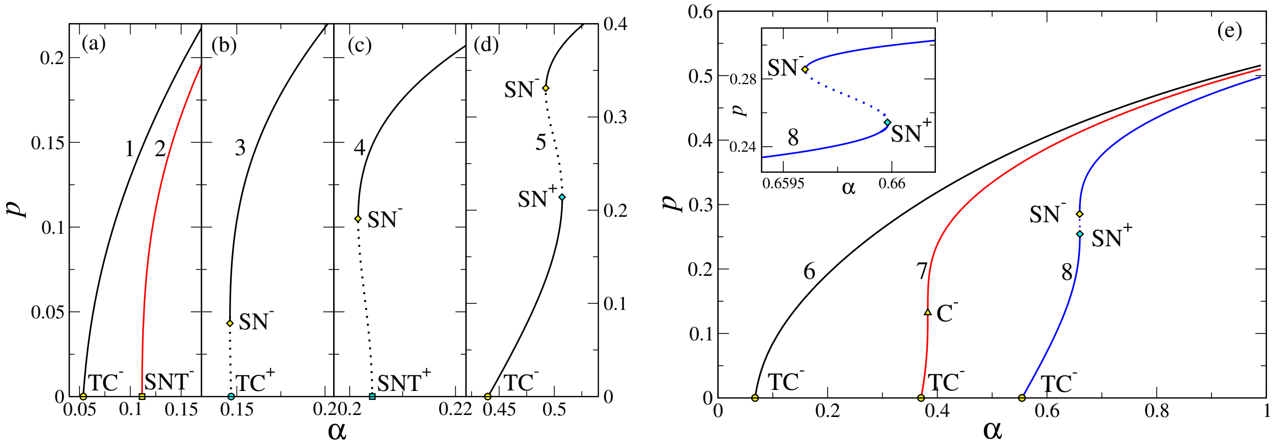


FIG. 3: The invasion curves for synergistic SIS epidemics spreading on the Douban network for the following sets of parameters $(\beta, \mu)$ indicated by numbered squares in Fig. 3(c). (a): $(\beta, \mu) = (-0.025, 0.5)$ for curve 1 and $(\beta, \mu) = (-0.04234, 0.5)$ for curve 2; (b): $(\beta, \mu) = (-0.05, 0.5)$; (c): $(\beta, \mu) = (-0.06064, 0.5)$; (d): $(\beta, \mu) = (-0.1, 0.5)$; (e): $(\beta, \mu) = (-0.025, 0.63)$ for curve 6, $(\beta, \mu) = (-0.07543, 0.63)$ for curve 7 and $(\beta, \mu) = (-0.1, 0.63)$ for curve 8. The inset in panel (e) shows the detailed part of the invasion curve 8 between two SN bifurcations indicated by circles with solid and dashed curves used for the stable and unstable states of the epidemic in this inset and in all other panels.

For d-time dynamics, the number of parameters is increased by one compared to c-time dynamics, and both SNT and C bifurcations of codimension-2 can occur. Their loci are shown by solid and dashed curves, respectively, in

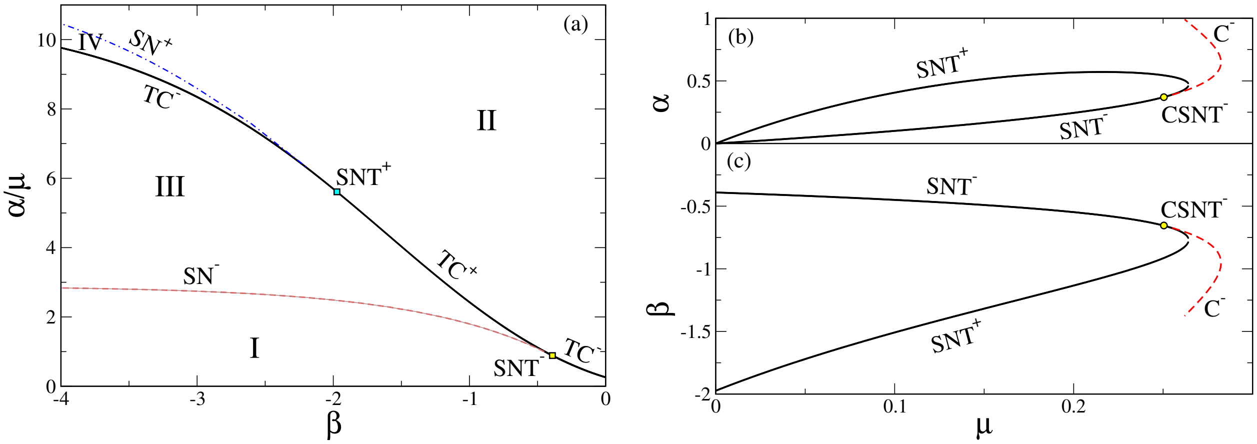


FIG. 4: Bifurcation diagrams for synergistic SIS epidemics spreading on the power grid network. Panel (a) displays the bifurcation diagram for c-time dynamics. Panels (b) and (c) show the bifurcation diagrams for d-time dynamics. The same line and symbol styles and notations for the bifurcation loci as in Fig. 2 are used in all panels.

$(\alpha, \mu)$ and $(\beta, \mu)$ parameter spaces displayed in panels (b) and (c) of Fig. 2. The C-bifurcation curve merges with the SNT-bifurcation curve at the codimension-3 bifurcation point called CSNT, i.e. cusp-(saddle-node-transcritical) collision point, shown by circles in Fig. 2(b)-(c). Similarly, as in the main text (see insets in Fig. 2 of the main text), the behaviour of SIS epidemics in the Douban network can be described and analysed in terms of the invasion curves (the curves for $p(\alpha)$) for different sets of parameters $\beta$ and $\mu$ labeled by the numbered squares in panel (c) of Fig. 2. The first set of invasion curves for $\mu = 0.5$ displayed in Fig. 3(a)-(d) demonstrates the behaviour of the epidemic in different regimes:

- Curve 1 in panel (a): the regime transition sequence, I-II, with increasing value of the base rate $\alpha$, i.e. epidemic evolves from the infection-free state ($p = 0$) to the endemic state (solid curve 1) through the $TC^-$ bifurcation labeled by circle (cf. with inset (i) in Fig.2(b) of the main text).

- Curve 2 in panel (a): the same regime sequence as for curve 1, but the transition occurs at the codimension-2 $SNT^-$ bifurcation labeled by square (not shown in the main text).

- Curve 3 in panel (b): the shape of the invasion curve is similar to that shown in inset (ii) in Fig.2(b) of the main text.

- Curve 4 in panel (c): the invasion curve is similar to curve 3 with $TC^+$ being replaced by $SNT^+$ (not shown in the main text).

- Curve 5 in pane (d): a similar behaviour as that shown in inset (vi) in Fig.2(d) of the main text.

The set of invasion curves 1-5 illustrates the evolution of the bifurcation points in terms of their number and type when the synergy strength increases in magnitude at a fixed value of $\mu$. Namely, for weak synergy, the system exhibits only a $TC^-$ bifurcation point (curve 1). With an increase of $|\beta|$, the $TC^-$ bifurcation transforms into $SNT^-$ (curve 2), giving rise to the $TC^+$ and $SN^-$ bifurcations (curve 3). A further increase in $|\beta|$ leads to the transformation of $TC^+$ into $SNT^+$ (curve 4), which in turn transforms into $TC^-$ and $SN^+$ bifurcations (curve 5).

The panel (e) of Fig. 3 shows the set of invasion curves 6-8 obtained at $\mu = 0.63$ and different values of $\beta$ (see the numbered squares on the right vertical dotted line in Fig. 2(c)). This panel (e) illustrates how the invasion curve with a single $TC^-$ bifurcation (curve 6) can transform to curve 7 with the $C^-$ bifurcation labeled by a triangle which then, in turn, transforms into curve 8 with two $SN^-$ and $SN^+$ bifurcations originating from the $C^-$ bifurcation.

Synergistic SIS epidemics spreading on the power grid network considered here exhibit bifurcation diagrams similar to those described above for the Douban network for both c- and d-time dynamics (see Fig. 4). This might be a consequence of relatively similar node degree distributions for both networks, which display some features of PL graphs.

## IV. MONTE CARLO SIMULATIONS OF SYNERGISTIC EPIDEMICS

In this section, we present the results of numerical Monte Carlo (MC) simulations for several model networks and compare them with the results obtained by using the SSHMF approximation. The model networks include ER, BG and PL (see Eq. (1) in the main text). Numerically, the networks were created by using an uncorrelated configuration model [4] and SIS run on the largest connected component of the ER and PL graphs.

### A. Binary graphs

It is expected that the results of MC simulations can support the mean-field analysis only at the qualitative rather than quantitative level, in a similar way to how it was demonstrated for synergistic SIS processes on $k$-regular random graphs [5]. The main reason for this is that the dynamical correlations are not captured by the SSHMF approximation. Indeed, the MC simulations reveal the same features observed in the SSHMF approximation, although the range of parameters corresponding to specific regimes of the SIS processes can differ between mean-field and exact numerical analysis. For example, all five mean-field dynamical regimes can be found in binary graphs BG$(10, 30, \varphi)$ for $\varphi \gtrsim 0.5$ but exact MC analysis demonstrates that only for $\varphi \gtrsim 0.6$ all five regimes can occur for synergistic SIS. Technically, the MC bifurcation diagrams were obtained by analyzing the roots of the rate function, as demonstrated in Ref. [5].

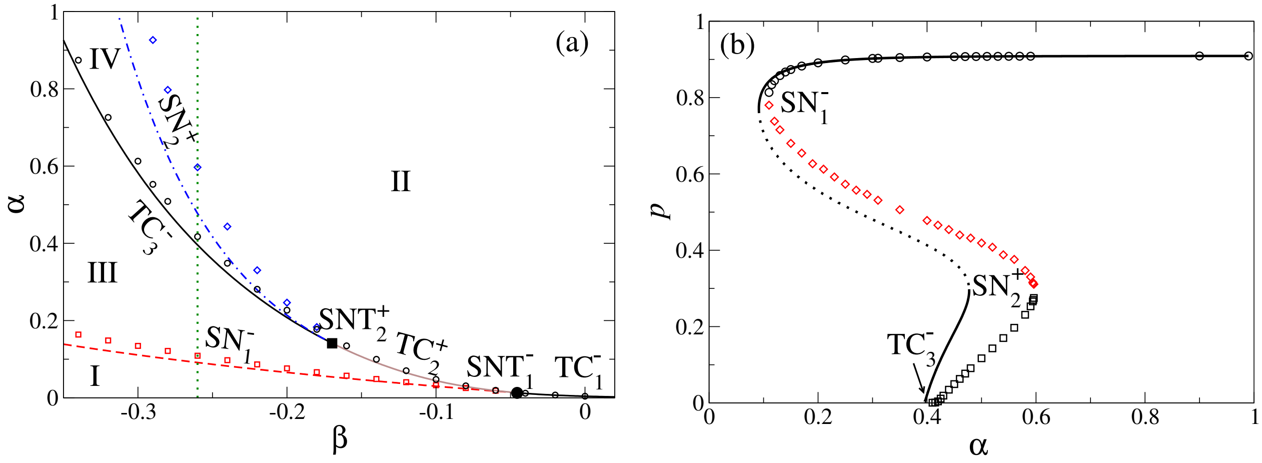


FIG. 5: In both panels, the curves and open symbols correspond to data obtained within the SSHMF approximation and by MC simulations, respectively. (a) Bifurcation diagram for synergistic SIS process on BG$(10, 30, \varphi)$ with $\varphi = 0.5$, and $\mu = 0.1$ (d-time). The finite-size networks containing $N = 10^5$ nodes were used in MC analysis. The dashed curve and open squares represent the line of $SN_1^-$ bifurcations separating regimes I and III. The dot-dashed curve and diamonds represent the line of $SN_2^+$ bifurcations separating regimes II and IV. The solid curve and circles correspond to: (i) $TC_1^-$ bifurcations separating regimes I and II for $\beta > \beta_{SNT_1^-}$, i.e. on the right of the saddle-node-transcritical crossing bifurcation $SNT_1^-$; (ii) $TC_2^+$ bifurcations separating regimes II and III for $\beta_{SNT_2^+} < \beta < \beta_{SNT_1^-}$; (iii) $TC_3^-$ bifurcations separating regimes III and IV for $\beta < \beta_{SNT_2^+}$. The solid circle and square refer to the mean-field data for $SNT_1^-$ and $SNT_2^+$ bifurcations, respectively.
(b) The proportion of infected nodes, $p$, in the high-endemic stable (top solid curve and circles), low-endemic stable (lower solid curve and squares) and unstable (dashed curve and diamonds) quasi-stationary states *vs* $\alpha$ for $\beta = -0.26$ (see the dotted vertical line in panel (a)) and the same values of other parameters as in panel (a).

We begin a comparative analysis between the mean-field and MC results obtained for synergistic SIS epidemics in BG$(10, 30, \varphi = 0.5)$ for $\mu = 0.1$ when four (rather than all five) regimes can occur within both approaches (see Fig. 5(a)). The data of numerical MC analysis shown by open symbols qualitatively support all the main features found within the SSHMF approximation, but the quantitative agreement is not perfect, as expected.

The shape of the invasion curve $p(\alpha)$ (see Fig. 5(b)) is similar to that shown in the inset (iii) of Fig. 2(b) in the main text. The numerical MC data (open symbols) reproduce well all the features on the invasion curve found within the SSHMF approximation (lines).

The numerical support of the bifurcation diagram that shows all five regimes with three SNT bifurcations is given in Fig. 6(a) for BG$(10, 30, \varphi = 0.7)$. The value of the parameter $\varphi = 0.7$ is chosen because the MC simulations for

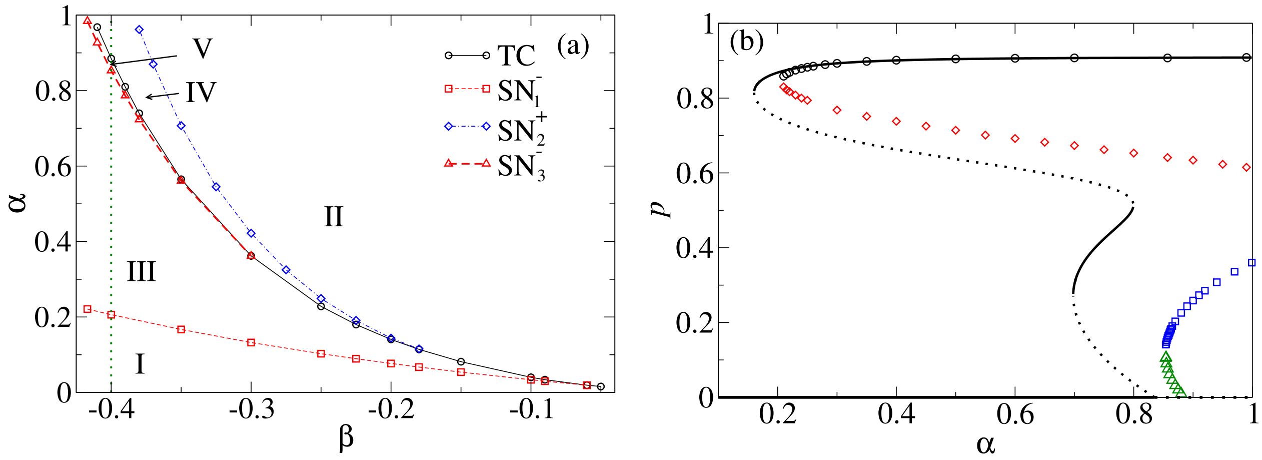


FIG. 6: (a) Bifurcation diagram for synergistic SIS process on BG$(10, 30, \varphi)$ ($N = 10^5$) with $\varphi = 0.7$, and $\mu = 0.1$ (d-time) obtained by MC simulations. The TC and SN bifurcations are shown by different symbols as indicated in the legend. The lines serve as a guide for the eye only. The error bars are smaller than the symbol size. (b) Symbols (solid and dotted lines) show the data for the invasion curve obtained by MC simulations (by SSHMF approximation) for $\beta = -0.4$ (see the vertical dotted line in panel (a)).

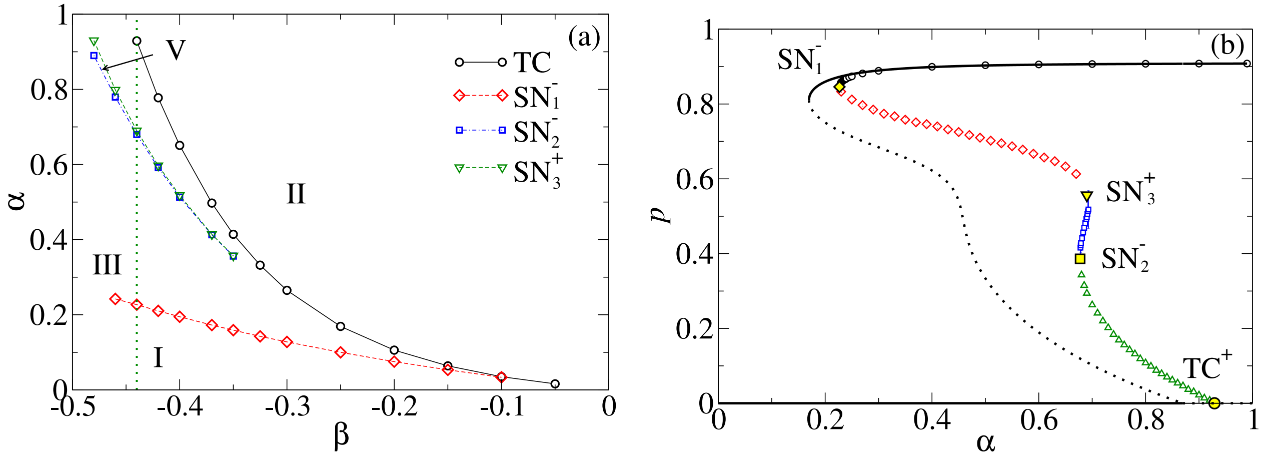


FIG. 7: (a) The MC bifurcation diagram for synergistic SIS process on BG$(10, 30, \varphi)$ ($N = 10^5$) with $\varphi = 0.82$ and $\mu = 0.1$ (d-time). The TC and SN bifurcations are shown by different symbols as indicated in the legend. The lines serve as a guide for the eye only. The error bars are smaller than the symbol size.
(b) Symbols (solid and dotted lines) show the data for the invasion curve obtained by MC simulations (by SSHMF approximation) for $\beta = -0.44$ and all other parameters being the same as for data in (a) (see the vertical dotted line in (a)). The solid and dotted lines correspond to the mean-field stable and unstable quasi-equilibrium states.

$\varphi = 0.6$ (as in Fig. 2(b) in the main text) do not exhibit all five regimes. The shape of the invasion curve shown in the inset (iv) of Fig. 2(b) in the main text is numerically supported by the MC and mean-field data in Fig. 6(b).

The numerical support for the bifurcation diagram and the invasion curve shown in the main text (main panel and inset of Fig. 2(c)) is given in panels (a) and (b) of Fig. 7, respectively. Fig. 7 displays the data for BG$(10, 30, \varphi = 0.82)$. The value of $\varphi = 0.82$ was chosen in the MC simulations in order to produce a bifurcation diagram similar to that displayed in Fig. 2(c) in the main text.

### B. Erdös-Rényi graphs

Bifurcation diagrams discussed in Sec. IV A for binary graphs are typical also for other networks characterised by continuous degree distributions although the type and number of bifurcations depends on the network topology. In

this subsection, we consider synergistic SIS spreading on classical random graphs with the Poisson degree distribution, i.e. Erdös-Rényi (ER) graphs.

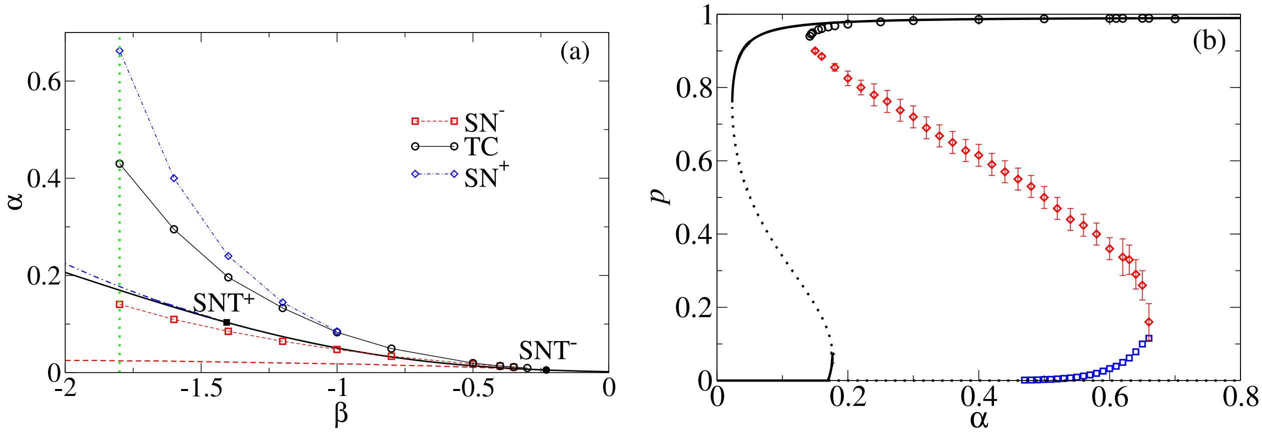


FIG. 8: (a) The bifurcation diagram for synergistic SIS on ER($\langle k\rangle$) graphs with $\langle k\rangle = 4$ and $\mu = 0.01$ (d-time). The SN$^-$, SN$^+$ and TC bifurcation lines are shown by dashed (open squares), dot-dashed (diamonds) and solid (circles) lines for the SSHMF (MC simulations, $N = 10^5$) data, respectively. The solid circle and square show the location of SNT$^-$ and SNT$^+$ bifurcations for the SSHMF data. The lines connecting the open symbols serve as eye-guides only. (b) The invasion curves for $\beta = -1.8$ (the vertical dotted line in (a)) obtained by MC simulations (symbols) and within the SSHMF approximation (solid and dotted curves). The solid and dotted curves refer to the stable and unstable quasi-equilibrium states of the SIS process.

ER graphs are characterized by a single network parameter $\Gamma_N = \langle k\rangle$, i.e. the mean degree. The synergistic SIS process on the ER graphs with $\langle k\rangle > 1$ can exhibit (within the SSHMF approximation) the following bifurcations: TC, SN, SNT, C and CSNT. For $\langle k\rangle \gtrsim 3.4$, only the TC, SN and SNT bifurcations occur with a maximum of two SNT bifurcations in the $(\alpha, \beta)$ plane for fixed $\mu$ and $\langle k\rangle$. A typical bifurcation diagram for $\langle k\rangle = 4$ and $\mu = 0.01$ (d-time dynamics) is shown in Fig. 8(a) and it is similar to that found for BG(10,30,$\varphi$) with $\varphi \lesssim 0.524$ and $\mu = 0.1$ (see Fig. 5(a)). The MC simulations run on the largest connected component of the ER graphs with appropriately renormalized degree distribution after removing the disconnected components qualitatively support (cf. open symbols with solid, dashed and dot-dashed curves in Fig. 5(a)) all the features found within mean-field approximation. Similarly, the shapes of the mean-field invasion curves are well reproduced by MC simulations as illustrated in Fig. 8(b) by an example of an invasion curve (cf. solid and dotted curves with the open symbols) similar to that displayed in the inset (iii) of Fig. 2(b) in the main text.

### C. PL graphs

The network parameters for the power-law (PL) graphs include $\Gamma_N = \{k_{\min}, k_{\max}, m\}$ (see Eq. (1) in the main text), and all types of bifurcations and bifurcation diagrams discussed in Sect. IV A can be found for the PL networks with $k_{\min} \geq 2$. For PL networks with $k_{\min} = 1$, only codimension-1, codimension-2 and CSNT bifurcations exist for synergistic SIS processes. As an illustration for PL(1,$k_{\max}, m$) graphs, in Fig. 9, we show an invasion curve (panel (a)) exhibiting a bi-stable regime V for synergistic SIS processes in the PL(1,50,2) (cf. inset (vi) in Fig. 2(d) of the main text). In fact, we analysed the SIS processes spreading on the largest connected component of the PL networks, but the degree distribution for such network exhibits only insignificant deviations from the power-law distribution for $k < 3$ (see the inset in Fig. 9(a)). Again, the MC simulations reproduce the mean-field shape of the invasion curve well (cf. open symbols with the solid curve in panel (a)).

The panel (b) of Fig. 9 provides a numerical support for the effect of heterogeneous infection (see Fig. 3 in the main text) which is clearly seen for the low-endemic stationary regimes II and IV, when the degree distribution of infected nodes is peak-shaped at relatively small values of $k$ (see the distributions obtained by MC simulations and marked by circles and squares for regime II and by diamonds for regime IV in panel (b)). This is in contrast to the high-endemic regime for which the degree distribution of infected nodes tends to uniform one (see the distributions marked by down-triangles for regime IV and up-triangles for regime II in (b)). The mean-field data for degree distributions of infected nodes agree with the MC data but only qualitatively (in panel (b), cf. the distributions $p_k^\infty$ marked by $\times$

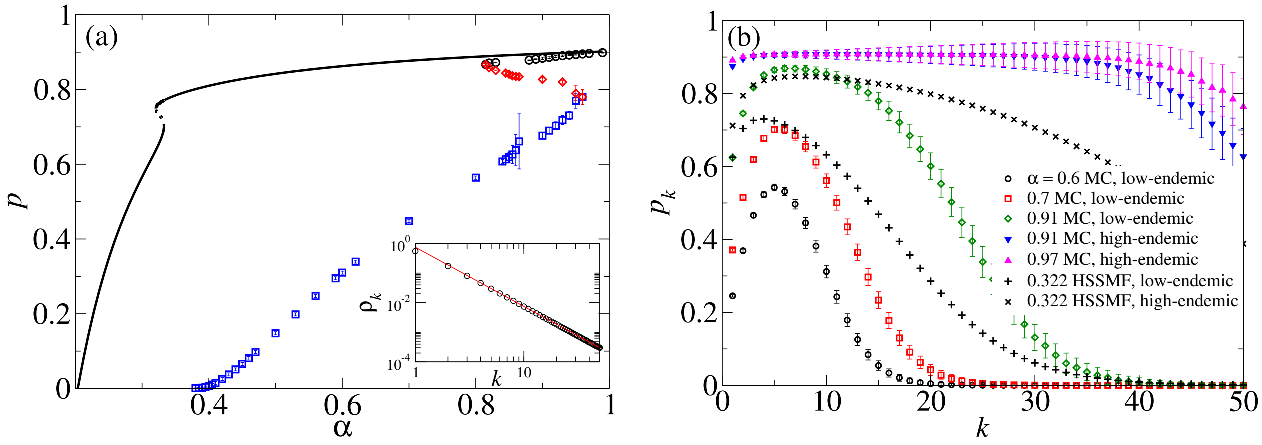


FIG. 9: (a) Invasion curves for synergistic SIS in the largest connected component of mean size $\langle N \rangle \simeq 83038$ in the PL(1,50,2) graph obtained by MC simulations (symbols) and by the HSSMP approximation (solid curve) for $\beta = -0.55$ and $\mu = 0.1$ (d-time). Blue squares, red diamonds and black circles refer to low-endemic, unstable and high-endemic MC stationary states, respectively. The degree distribution, $\rho_k$, for the largest connected component in PL(1,50,2) networks is shown by circles in the inset (the solid line shows $\rho_k \propto k^{-2}$ for reference). (b) Degree distributions of the infected nodes obtained by MC simulations for the low-endemic (open symbols) and high-endemic (solid symbols) states for different values of $\alpha$ as indicated in the legend. The degree distributions of the infected nodes obtained within the SSHMF approximation are depicted by + (for the low-endemic states) and $\times$ (for the high-endemic states).

and + with those obtained by MC calculations).


[1] T. M. Apostol, *Mathematical Analysis*, 2nd ed. (Reading, Mass., Addison-Wesley Pub. Co., 1974).
[2] J. Kunegis, in *Proc. Int. Conf. on World Wide Web Companion* (2013) pp. 1343–1350.
[3] R. A. Rossi and N. K. Ahmed, in *AAAI* (2015) pp. 4292–4293.
[4] M. Catanzaro, M. Boguñá, and R. Pastor-Satorras, Phys. Rev. E **71**, 027103 (2005).
[5] S. N. Taraskin and F. J. Pérez-Reche, Journal of Physics A: Mathematical and Theoretical **52**, 195101 (2019).
